# Supplementary material for: Long Video Generation with Time-Agnostic VQGAN and Time-Sensitive Transformer
Source: arXiv:2204.03638 source file (2022-09-24)
Supplement: Supplementary file 1 [file eccv2022supplementary.tex]

% updated April 2002 by Antje Endemann
% Based on CVPR 07 and LNCS, with modifications by DAF, AZ and elle, 2008 and AA, 2010, and CC, 2011; TT, 2014; AAS, 2016; AAS, 2020; TH, 2022

% \documentclass{article}
\documentclass[runningheads]{llncs}
\usepackage{graphicx}
% DO NOT USE \usepackage{times}, it will be removed by typesetters
%\usepackage{times}

\usepackage{tikz}
\usepackage{comment}
\usepackage{amsmath,amssymb} % define this before the line numbering.
\usepackage{color}
\usepackage[utf8]{inputenc}

% The "axessiblity" package can be found at: https://ctan.org/pkg/axessibility?lang=en
\usepackage[accsupp]{axessibility}  % Improves PDF readability for those with disabilities.

% INITIAL SUBMISSION - The following two lines are NOT commented
% CAMERA READY - Comment OUT the following two lines
% \usepackage{ruler}
% \usepackage[width=122mm,left=12mm,paperwidth=146mm,height=193mm,top=12mm,paperheight=217mm]{geometry}

\usepackage{booktabs}

\usepackage{url}
\usepackage{subcaption}
\usepackage[pagebackref=true,breaklinks=true,letterpaper=true,pagebackref=true,colorlinks,bookmarks=false]{hyperref}

\usepackage{wrapfig}

\usepackage{pifont}% http://ctan.org/pkg/pifont

\begin{document}
% \renewcommand\thelinenumber{\color[rgb]{0.2,0.5,0.8}\normalfont\sffamily\scriptsize\arabic{linenumber}\color[rgb]{0,0,0}}
% \renewcommand\makeLineNumber {\hss\thelinenumber\ \hspace{6mm} \rlap{\hskip\textwidth\ \hspace{6.5mm}\thelinenumber}}
% \linenumbers
\pagestyle{headings}
\mainmatter
\def\ECCVSubNumber{5950}  % Insert your submission number here

\title{Supplementary Material of Long Video Generation with Time-Agnostic VQGAN and Time-Sensitive Transformer}

% INITIAL SUBMISSION 
\begin{comment}
\titlerunning{ECCV-22 submission ID \ECCVSubNumber} 
\authorrunning{ECCV-22 submission ID \ECCVSubNumber} 
\author{Anonymous ECCV submission}
\institute{Paper ID \ECCVSubNumber}
\end{comment}
%******************

% CAMERA READY SUBMISSION
% \begin{comment}
\titlerunning{Supplementary Material of TATS}
% If the paper title is too long for the running head, you can set
% an abbreviated paper title here
% %
\author{}
\institute{}
% \author{Songwei Ge\inst{1}\thanks{Work done primarily during an internship at Meta AI.} \and
% Thomas Hayes\inst{2} \and
% Harry Yang\inst{2} \and
% Xi Yin\inst{2} \and
% Guan Pang\inst{2} \\
% David Jacobs\inst{1} \and
% Jia-Bin Huang\inst{1,2} \and
% Devi Parikh\inst{2,3}}
% %
\authorrunning{S. Ge, T. Hayes, H. Yang, X. Yin, G. Pang, D. Jacobs, J. Huang, D. Parikh}
% % First names are abbreviated in the running head.
% % If there are more than two authors, 'et al.' is used.
% %
% \institute{\textsuperscript{1}University of Maryland \hspace{0.2cm} \textsuperscript{2}Meta AI \hspace{0.2cm} \textsuperscript{3}Georgia Tech}
% \email{\{songweig,djacobs\}@umd.com, \{thayes427,harryyang,yinxi,gpang,jbhuang,dparikh\}@fb.com}}
% \end{comment}
%******************
\maketitle

% \tableofcontents

\appendix
\addtocounter{figure}{9}
\input{sections/6_appendix}

\clearpage
% ---- Bibliography ----
%
% BibTeX users should specify bibliography style 'splncs04'.
% References will then be sorted and formatted in the correct style.
%
\bibliographystyle{splncs04}
\bibliography{egbib}
\end{document}
